# Supplementary material for: Hydrodynamic finite-size scaling of the thermal conductivity in glasses
Source: arXiv:2303.07010 ancillary file (2023-09-01)
Supplement: Supplementary file 1 [file SI.pdf]

# Supplementary Information to *Hydrodynamic finite-size scaling of the thermal conductivity in glasses*

Alfredo Fiorentino<sup>1</sup>, Paolo Pegolo<sup>1</sup> and Stefano Baroni<sup>1,2</sup>

<sup>1</sup>SISSA—Scuola Internazionale Superiore di Studi Avanzati, 34136 Trieste, Italy, European Union

<sup>2</sup>CNR-IOM—Istituto Officina Materiali, SISSA Unit, 34136 Trieste, Italy, European Union

(Dated: September 1, 2023)

## Supplementary Note 1. COMPARISON OF THE HYDRODYNAMIC EXTRAPOLATION WITH OTHER METHODS

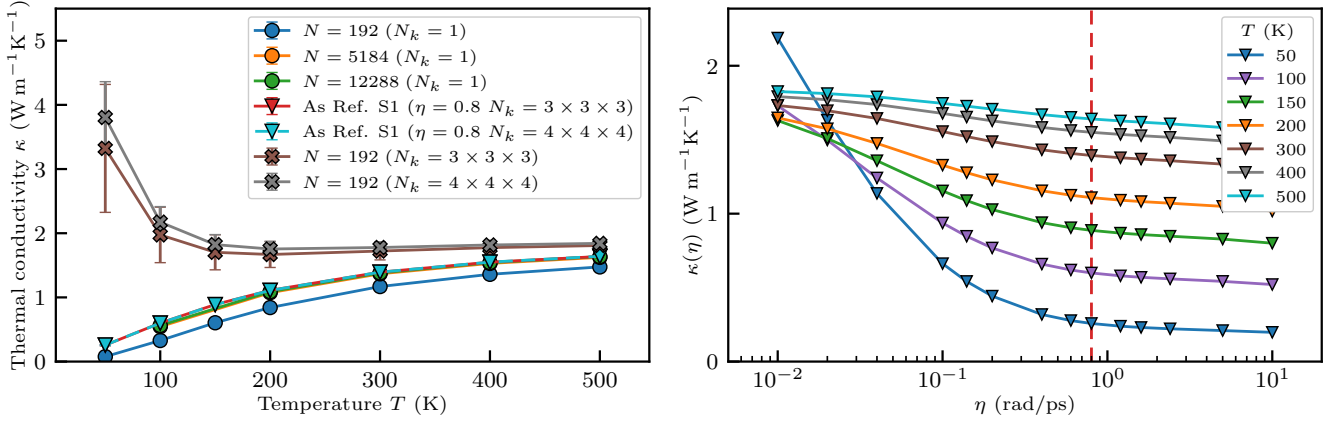

Supplementary Figure 1. Application of the method of Supplementary Reference 1 to the computation of the thermal conductivity of  $a\text{SiO}_2$ . The left panel shows  $\kappa$  as a function of temperature for the different cases explained in the text; the right panel shows  $\kappa$  computed on a  $3 \times 3 \times 3$   $q$ -mesh as a function of the regularization parameter,  $\eta$ , and for different temperatures.

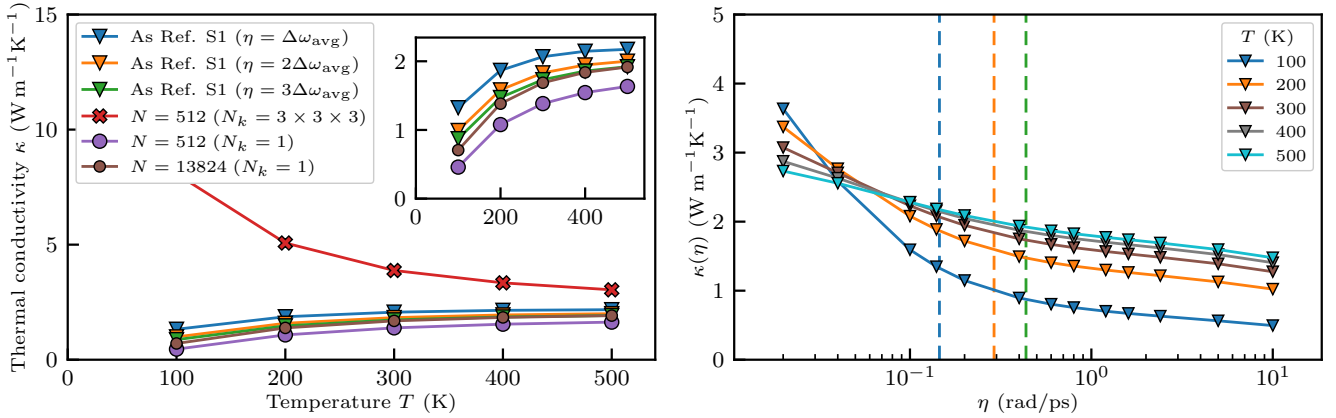

Supplementary Figure 2. Application of the method of Supplementary Reference 1 to the computation of the thermal conductivity of  $a\text{SiC}$ . The left panel shows  $\kappa$  as a function of temperature for the different cases explained in the text; the right panel shows  $\kappa$  computed on a  $3 \times 3 \times 3$   $q$ -mesh as a function of the regularization parameter,  $\eta$ , and for different temperatures.

We provide some details on calculations made according to the regularization protocol of Supplementary Reference 1, reviewed in the main text. The actual implementation of the regularization protocol is the one outlined in the main text, i.e., a finite width  $\eta/2$  is added to each anharmonic linewidth of the normal modes of the crystallized sample. In amorphous silica ( $a\text{SiO}_2$ , Supplementary Figure 1), the method reproduces what is found in Supplementary

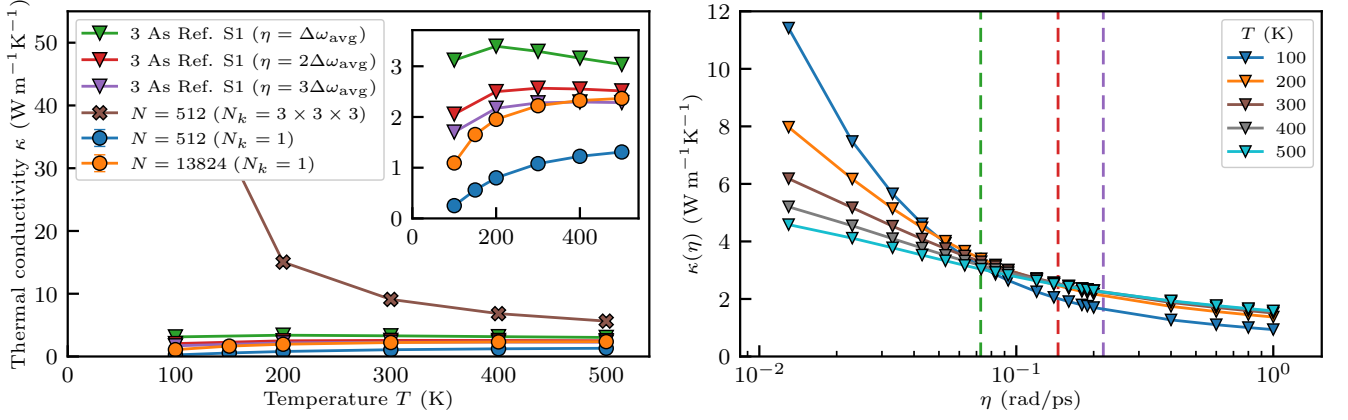

Supplementary Figure 3. Application of the method of Supplementary Reference 1 to the computation of the thermal conductivity of *aSi*. The left panel shows  $\kappa$  as a function of temperature for the different cases explained in the text; the right panel shows  $\kappa$  computed on a  $3 \times 3 \times 3$   $q$ -mesh as a function of the regularization parameter,  $\eta$ , and for different temperatures.

Reference 1, i.e., the regularized thermal conductivity of a small sample with  $N$  atoms computed on an  $\ell \times \ell \times \ell$  mesh in the Brillouin Zone (BZ) is compatible with that of a genuinely disordered system with  $\ell^3 N$  atoms obtained from calculations made at the BZ center alone. As explained in the main text, the same is not true for amorphous silicon carbide (*aSiC*, Supplementary Figure 2) and amorphous silicon (*aSi*, Supplementary Figure 3). In fact, no plateau is found in the thermal conductivity of these two materials as a function of  $\eta$ , thus making it impossible to find a suitable value for that parameter able to bridge the value of  $\kappa$  of the small, crystallized, sample with the one of the larger, genuinely disordered, one.

We show the results of the application of the method of Supplementary Reference 1 to the computation of thermal conductivity of *aSiO<sub>2</sub>*, *aSiC* and *aSi* respectively in Supplementary Figure 1,2 and 3. For each figure, the left panel shows  $\kappa$  as a function of temperature for different cases: the circles are results computed at the BZ center for different sizes, the crosses are computed on a  $3 \times 3 \times 3$  or  $4 \times 4 \times 4$   $q$ -mesh starting from the smallest size so that the equivalent number of atoms is the same as the large sample at the  $\Gamma$  point. The triangles are computed on the dense  $q$ -mesh but regularized by  $\eta$ . For *aSiO<sub>2</sub>* we choose  $\eta$  according to Supplementary Reference 1 in correspondence with the plateau indicated in the right panel by a red dashed vertical line. For each material, the right panel presents  $\kappa$  computed on a  $3 \times 3 \times 3$   $q$ -mesh as a function of  $\eta$  for different temperatures. For *aSiC* and *aSi* we can not find any plateau. Therefore we just show in the left panel the results for three reasonable values of  $\eta$ , i.e. integer multiples,  $m = 1, 2, 3$ , of the average spacing,  $\eta = m\Delta\omega_{\text{avg}}$ , where  $\Delta\omega_{\text{avg}} = \omega_{\text{max}}/3N_{\text{atoms}}$ . These three values correspond to the three vertical lines in the right panel. We observe a significative difference between these three lines, depending on the value of  $\eta$ .

## Supplementary Note 2. GREEN-KUBO MOLECULAR DYNAMICS

The size scaling of the thermal conductivity in *aSi* is assessed through large Green-Kubo Molecular Dynamics (GKMD) simulations. The simulations are carried out with the **GPUMD** code [2], where the energy flux is properly implemented for the Tersoff force-field [3]. Each thermal conductivity value is obtained through the Helfand-Einstein integration [4, 5] of the energy flux autocorrelation function. The flux is sampled every 2 fs from a canonical dynamics controlled by the Bussi-Donadio-Parrinello thermostat [6]. The results are shown in Supplementary Figure 4. Even for  $\ell = 20$ , i.e. for systems with 64000 atoms, the value of  $\kappa$  is not at convergence. This agrees with the fact that models with 13824 atoms are still far from convergence in our QHGK calculations, and the hydrodynamic extrapolation is helpful in achieving a converged value of  $\kappa$  through affordable QHGK simulations.

## Supplementary Note 3. CHOICE OF THE CUTOFF FREQUENCY FOR PROPAGONS

In the main text the choice of the cutoff (angular) frequency of propagons,  $\omega_P$ , is explained in terms of the Ioffe-Regel limit and the propagon dispersion. However, the primary criterion is that the model should be valid for the frequency range determined by  $\omega_P$ . Specifically, below  $\omega_P$ , the VDOS should exhibit quadratic behavior, and the

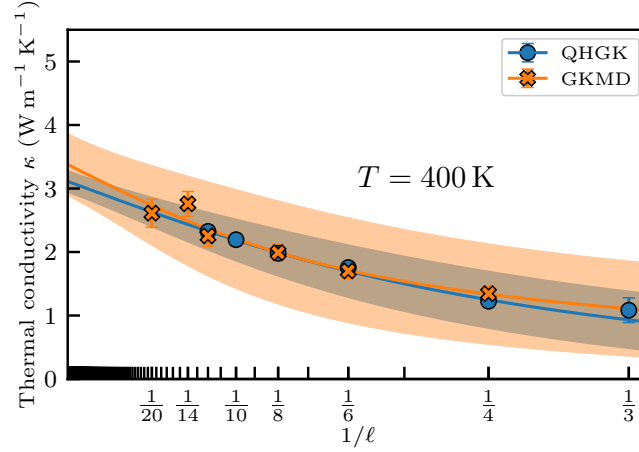

Supplementary Figure 4. Comparison of the size scaling of  $\kappa$  in  $a\text{Si}$  from QHGK calculations and GKMD simulations at 400 K. Even for  $\ell = 20$ , i.e. for systems with 64000 atoms, the convergence in size is yet to be achieved. The error bars of the GKMD data are obtained through standard block-averaging of 10 ns-long time series of four different samples for each size; the error bars of the QHGK data are standard deviations over ten different samples for each size. The solid lines are fitted according to Equation (24) in the main text. The shaded areas indicate the error in the fit, obtained by propagating the covariance matrix of the fitting parameters under the assumption of independent variables.

linewidths of the two branches should be sufficiently small to prevent mixing between them. As these conditions do not precisely define a sharp criterion for choosing the appropriate value of  $\omega_P$ , this section provides some suggestions in this regard.

Initially, a tentative choice can be made based on the linearity of the dispersion and avoidance of mixing. This can be accomplished by visually examining a plot of the VDSF. Once a tentative value is obtained, it is advisable to slightly alter the chosen value and observe the resulting change in  $\kappa$ . The variation in  $\kappa$  primarily depends on how the linewidths fit is affected by the change in  $\omega_P$ . In practice, reasonable values of  $\omega_P$  would only include a small number of frequencies below this threshold, resulting in a limited number of data points for fitting. Notably, the longitudinal branch, with its higher sound velocity, exacerbates this issue by having fewer frequencies below the cutoff compared to the transverse branches. Therefore, meaningful variations of  $\omega_P$  should involve at least one longitudinal frequency.

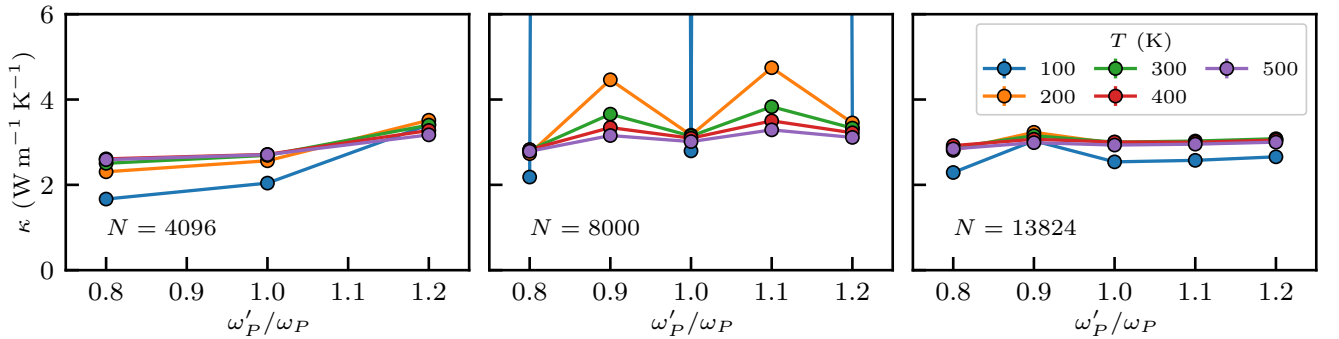

Supplementary Figure 5. Dependence of the thermal conductivity on the propagon cutoff angular frequency.

In Supplementary Figure 5, we present some tests conducted on  $a\text{Si}$  to compute the thermal conductivity for various temperatures, as a function of the cutoff angular frequency. The reference value is  $\omega_P/2\pi = 3$ , THz, and  $\omega'_P$  is allowed to vary from  $0.8, \omega_P$  to  $1.2, \omega_P$ . For  $N = 4096$ , transitioning from  $0.8, \omega_P$  to  $\omega_P$  and from  $\omega_P$  to  $1.2, \omega_P$  only introduces one additional frequency. Consequently, displaying values like  $0.9, \omega_P$  would be meaningless. The same applies to finer meshes at larger sizes.

It should be noted that, for  $N = 8000$ , selecting a cutoff of  $0.9, \omega_P$  or  $1.1, \omega_P$  yields extremely large values of  $\kappa$ . This suggests that, in some cases, the fitting procedure may be unstable even with the inclusion of a single data point.

Although this finding is somewhat concerning, it is worth mentioning that a slight adjustment to the cutoff frequency results in a sensible value of  $\kappa$ . Nevertheless, this situation emphasizes the need for the development of alternative methods that offer greater stability and reduce dependence on the choice of  $\omega_P$ . Work is being done in this direction.

### SUPPLEMENTARY REFERENCES

---

- [1] M. Simoncelli, F. Mauri, and N. Marzari, Thermal conductivity of glasses: first-principles theory and applications, *NPJ Comput. Mater.* **9**, 106 (2023).
- [2] Z. Fan, Y. Wang, P. Ying, K. Song, J. Wang, Y. Wang, Z. Zeng, K. Xu, E. Lindgren, J. M. Rahm, *et al.*, Gpumd: A package for constructing accurate machine-learned potentials and performing highly efficient atomistic simulations, *J. Chem. Phys.* **157**, 114801 (2022).
- [3] Z. Fan, L. F. C. Pereira, H.-Q. Wang, J.-C. Zheng, D. Donadio, and A. Harju, Force and heat current formulas for many-body potentials in molecular dynamics simulations with applications to thermal conductivity calculations, *Phys. Rev. B* **92**, 094301 (2015).
- [4] S. Baroni, R. Bertossa, L. Ercole, F. Grasselli, and A. Marcolongo, Heat transport in insulators from ab initio green-kubo theory, *Handbook of materials modeling: Applications: Current and emerging materials*, 809 (2020).
- [5] F. Grasselli and S. Baroni, Invariance principles in the theory and computation of transport coefficients, *Eur. Phys. J. B* **94**, 1 (2021).
- [6] G. Bussi, D. Donadio, and M. Parrinello, Canonical sampling through velocity rescaling, *J. Chem. Phys.* **126**, 014101 (2007).
